# Supplementary material for: Kinematic Base State Estimation for Humanoid using Invariant Extended Kalman Filter
Source: arXiv:2401.02786 source file (2024-01-05)
Supplement: Supplementary file 1 [file appendix.tex]

when dealing with the rotation matrix, we employ the following formulation:
\begin{equation}\label{eq:410}
	\pmb{R}_{k+1} = \pmb{R}_k exp(\bar{\pmb{\omega}}^\wedge \Delta t)
\end{equation}
Once the orientation equations have been determined, the next step involves integrating equations 7 and 8 to derive the discrete equations for velocity and position.
\begin{align}\label{eq:445}
    \pmb{v}_{k+1} = & \pmb{v}_k + \int_{t_k}^{t_{k+1}} \pmb{R}_{k+1} \bar{\pmb{a}} + \pmb{g} dt = \nonumber \\
&\pmb{v}_k + \pmb{g} \Delta t + \pmb{R}_k(\int_{t_k}^{t_{k+1}} exp(\bar{\pmb{\omega}}^\wedge t) dt)\bar{\pmb{a}}
\end{align}
\begin{equation}\label{eq:410}
	\pmb{p}_{k+1} = \pmb{p}_k + \pmb{v}_k \Delta t + \frac{1}{2} \pmb{g} \Delta t^2 + 
\pmb{R}_k(\int_{t_k}^{t_{k+1}} \int_{t_k}^{\tau} exp(\bar{\pmb{\omega}}^\wedge t) dt d\tau)\bar{\pmb{a}}
\end{equation}
